# Supplementary material for: DeltaLCA: Comparative Life-Cycle Assessment for Electronics Design
Source: arXiv:2311.09611 source file (2023-11-16)
Supplement: Supplementary file 1 [file supplementart-materials.tex]

There are three supplementary materials:

1- "orientation-slides.pdf" is a PDF containing the orientation presentation during user studies. 

2- "post-study-questionnaire.pdf" is a PDF that contains the pre-study questionnaire questions.

3- "post-study-questionnaire.pdf" is a PDF that contains the post-study questionnaire questions.
